# Supplementary material for: An accurate and efficient framework for modelling the surface chemistry of ionic materials
Source: arXiv:2412.17204 source file (2025-04-11)
Supplement: Supplementary file 1 [file SI_Table-Erlx_MgO.tex]

\begin{table}
\caption{\label{tab:lattice_parameters_mgo}Relaxation energy $E_\text{rlx}$ (in meV) for the adsorbate--surface systems with the MgO surface obtained from the DFT ensemble.}
\begin{tabular}{lrrrrrr}
\toprule
 & PBE-D2[Ne] & revPBE-D4 & vdW-DF & rev-vdW-DF2 & PBE0-D4 & B3LYP-D2[Ne] \\ 
\midrule
CH$_4$ on MgO(001) & 4 & 2 & 0 & 2 & 0 & 0 \\
Monolayer CH$_4$ on MgO(001) & 3 & 1 & 0 & 2 & -2 & -1 \\
C$_2$H$_6$ on MgO(001) & 3 & 1 & -2 & 2 & -4 & -3 \\
Monolayer C$_2$H$_6$ on MgO(001) & 4 & 4 & 1 & 2 & -4 & -1 \\
CO on MgO(001) & 13 & 8 & 13 & 13 & 9 & 11 \\
C$_6$H$_6$ on MgO(001) & 24 & 26 & 11 & 18 & 6 & 7 \\
Parallel N$_2$O on MgO(001) & 5 & 3 & 4 & 6 & 2 & 4 \\
Tilted N$_2$O on MgO(001) & 9 & 10 & 3 & 11 & 7 & 6 \\
Vertical-Hollow NO on MgO(001) & 75 & 29 & 13 & 62 & 2 & 3 \\
Vertical-Mg NO on MgO(001) & 10 & 9 & 9 & 48 & 5 & 5 \\
Bent-Bridge NO on MgO(001) & 49 & 51 & 33 & 51 & 13 & 9 \\
Bent-Mg NO on MgO(001) & 7 & 6 & 7 & 7 & 2 & 2 \\
Bent-O NO on MgO(001) & 39 & 39 & 18 & 39 & 3 & 5 \\
Dimer NO on MgO(001) & 54 & 42 & 46 & 54 & 20 & 26 \\
Monomer H$_2$O on MgO(001) & 131 & 114 & 90 & 134 & 121 & 113 \\
Tetramer H$_2$O on MgO(001) & 60 & 52 & 51 & 60 & 59 & 58 \\
Tilted CH$_3$OH on MgO(001) & 163 & 145 & 102 & 152 & 141 & 132 \\
Parallel CH$_3$OH on MgO(001) & 48 & 46 & 26 & 43 & 41 & 35 \\
Tetramer CH$_3$OH on MgO(001) & 79 & 68 & 58 & 75 & 69 & 75 \\
NH$_3$ on MgO(001) & 99 & 89 & 103 & 95 & 106 & 115 \\
Physisorbed CO$_2$ on MgO(001) & 15 & 14 & 6 & 16 & 10 & 9 \\
Chemisorbed CO$_2$ on MgO(001) & 693 & 663 & 704 & 676 & 773 & 810 \\
\bottomrule
\end{tabular}
\end{table}
