# Supplementary material for: An accurate and efficient framework for modelling the surface chemistry of ionic materials
Source: arXiv:2412.17204 source file (2025-04-11)
Supplement: Supplementary file 2 [file SI_Table-Erlx_TiO2.tex]

\begin{table}
\caption{\label{tab:lattice_parameters_tio2}Relaxation energy $E_\text{rlx}$ (in meV) for the adsorbate--surface systems with the \ce{TiO2} surfaces obtained from the DFT ensemble.}
\begin{tabular}{lrrrrrr}
\toprule
 & PBE-TS/HI & revPBE-D4 & vdW-DF & rev-vdW-DF2 & r$^2$SCAN-rVV10 & HSE06-D4 \\ 
\midrule
CH$_4$ on TiO$_2$ rutile(110) & 15 & 22 & 5 & 27 & 44 & 26 \\
Parallel CO$_2$ on TiO$_2$ rutile(110) & 25 & 14 & 17 & 30 & 32 & 30 \\
Tilted CO$_2$ on TiO$_2$ rutile(110) & 35 & 50 & 37 & 72 & 92 & 78 \\
H$_2$O on TiO$_2$ rutile(110) & 294 & 238 & 177 & 295 & 320 & 318 \\
CH$_3$OH on TiO$_2$ rutile(110) & 360 & 302 & 266 & 363 & 379 & 390 \\
H$_2$O on TiO$_2$ anatase(101) & 235 & 225 & 157 & 246 & 267 & 257 \\
NH$_3$ on TiO$_2$ anatase(101) & 223 & 212 & 194 & 223 & 237 & 247 \\
\bottomrule
\end{tabular}
\end{table}
